# Supplementary material for: Detecting Dataset Abuse in Fine-Tuning Stable Diffusion Models for Text-to-Image Synthesis
Source: arXiv:2409.18897 source file (2024-09-27)
Supplement: Supplementary file 1 [file appendix.tex]

\section{Overflow form other sections}
\label{sec:set-diff-dodis}
